# Supplementary material for: Real-Time Parallel Trajectory Optimization with Spatiotemporal Safety Constraints for Autonomous Driving in Congested Traffic
Source: arXiv:2309.05298 source file (2023-09-11)
Supplement: Supplementary file 1 [file appendix.tex]

\appendix
\subsection{Matrix definitions}\label{app:matrices}
  \footnotesize
